# Supplementary material for: Novel observation of isospin structure of short-range correlations in calcium isotopes
Source: arXiv:2004.11448 source file (2020-12-17)
Supplement: Supplementary file 1 [file Supplementary_V6.pdf]

# Supplementary Materials: Novel observation of isospin structure of short-range correlations in Calcium isotopes

## 1. SHORT-RANGE CORRELATION (SRC) MODEL

We use a simple model to interpret the measured per-nucleon cross section ratio in term of relative np, pp and nn SRC contributions. Our model takes into account the number of each type of NN pairs as well as two additional parameters, $f_{sr}(A)$ and $p_{NN}$, that account for of nucleons being close enough together to have a hard interaction, and the impact of isospin structure of the short-range NN interaction. The quantity $f_{sr}(A)$ is probability for any two nucleons to be close enough together to interact via the short-range NN interaction for a given nucleus and is assumed to be the same for np, pp, nn. The quantity $p_{NN}$ is probability that the NN interaction generates a high-momentum pair between the nucleons that are close together. This depends on the range of initial momentum $\Delta P_i$ and is taken to be the same for pp and nn pairs but different for nn pairs. For a given nuclear A(Z,N), the number of pp, np, and nn SRCs can be calculated as follows:

$$N_{np} = N \cdot Z \cdot f_{sr}(A) \cdot p_{np}(\Delta P_i) \tag{1}$$
$$N_{pp} = Z \cdot (Z-1)/2 \cdot f_{sr}(A) \cdot p_{pp}(\Delta P_i) \tag{2}$$
$$N_{nn} = N \cdot (N-1)/2 \cdot f_{sr}(A) \cdot p_{pp}(\Delta P_i) \tag{3}$$

### 1.1. Inclusive cross section ratios

Then contribution of these SRCs to the inclusive cross section in the 2N-SRC dominated region is:

$$\sigma_{np} = N \cdot Z \cdot f_{sr}(A) \cdot p_{np} \cdot (\sigma_{ep} + \sigma_{en}) \tag{4}$$
$$\sigma_{pp} = \frac{Z \cdot (Z-1)}{2} \cdot f_{sr}(A) \cdot p_{pp} \cdot (2\sigma_{ep}) \tag{5}$$
$$\sigma_{nn} = \frac{N \cdot (N-1)}{2} \cdot f_{sr}(A) \cdot p_{pp} \cdot (2\sigma_{en}) \tag{6}$$

where the cross section for quasielastic scattering from one of the nucleons is taken as the elastic e-N cross section at the $Q^2$ of the interaction.

The total cross section is then the sum of these three contributions:

$$\sigma_A = f_{sr}(A) \cdot \sigma_{en} \cdot p_{pp} \cdot \Big( N \cdot Z(1 + \frac{\sigma_{ep}}{\sigma_{en}}) \cdot \frac{p_{np}}{p_{pp}} + Z \cdot (Z-1) \cdot \frac{\sigma_{ep}}{\sigma_{en}} + N \cdot (N-1) \Big) \tag{7}$$
$$= f_{sr}(A) \cdot \sigma_{en} \cdot p_{pp} \cdot (\alpha \cdot R + \beta) \tag{8}$$

where the average value of $r = \frac{\sigma_{ep}}{\sigma_{en}}$ is 2.55-2.6 for the kinematic of this experiment, $R = \frac{p_{np}}{p_{pp}}$, and

$$\alpha = N \cdot Z \cdot (1 + r) \quad \text{and} \quad \beta = Z \cdot (Z-1) \cdot r + N \cdot (N-1)$$

The cross section ratio for two nuclei is then:

$$\frac{\sigma_{A_1}}{\sigma_{A_2}} = \frac{f_{sr}(A_1) \cdot \sigma_{en} \cdot p_{pp} \cdot (\alpha_1 \cdot R + \beta_1)}{f_{sr}(A_2) \cdot \sigma_{en} \cdot p_{pp} \cdot (\alpha_2 \cdot R + \beta_2)} = \frac{f_{sr}(A_1) \cdot (\alpha_1 \cdot R + \beta_1)}{f_{sr}(A_2) \cdot (\alpha_2 \cdot R + \beta_2)} \tag{9}$$

Taking $\frac{f_{sr}(A_1)}{f_{sr}(A_2)} = \frac{A_2}{A_1}$, the per-nucleon cross section ratio becomes

$$\frac{\sigma_{A_1}/A_1}{\sigma_{A_2}/A_2} = \frac{A_2^2}{A_1^2} \cdot \frac{(\alpha_1 \cdot R + \beta_1)}{(\alpha_2 \cdot R + \beta_2)}. \tag{10}$$

Taking $A_1, A_2$ to be $^{48}$Ca and $^{40}$Ca, respectively, and assuming isospin independence ($R = \frac{p_{pn}}{p_{pp}} = 1$), yields

$$\frac{\sigma_{^{48}\mathrm{Ca}}/48}{\sigma_{^{40}\mathrm{Ca}}/40} = 0.930. \tag{11}$$

Assuming complete np dominance, corresponding to taking $R \to \infty$, the cross section ratio is

$$\frac{\sigma_{^{48}\mathrm{Ca}}/48}{\sigma_{^{40}\mathrm{Ca}}/40} = 0.972. \tag{12}$$

corresponding to the limits provided in the paper. To extract R from the measurement, one simply needs to solve Equation ?? for R given the measurement of the per-nucleon cross section ratio.

### 1.2. Triple-coincidence measurements

The triple-coincidence experiments measure A(e,e'p) scattering corresponding to a proton with a large initial momentum, and look for a spectator nucleon from the SRC (with a momentum roughly opposite to that of the initial proton momentum). The then apply corrections to estimate the number of pp-SRCs to np-SRCs in the initial state. In our model, this ratio is:

$$\frac{\#\text{ pp-SRC}}{\#\text{ np-SRC}} = \frac{N_{pp}\cdot f_{sr}(A)\cdot p_{pp}}{N_{np}\cdot f_{sr}(A)\cdot p_{np}} = \frac{Z(Z-1)/2\cdot p_{pp}}{NZ\cdot p_{np}} = \frac{(Z-1)}{2N}R \tag{13}$$

where $p_{pp}$ and $p_{np}$ correspond to the $\Delta P_i$ range defined by the A(e,e'p) acceptance. This allows for the extraction of $R$ directly from the quoted ratio of pp to np pairs.

## 2. CALCIUM CROSS-SECTIONS AND $^{48}$CA/$^{40}$CA RATIOS

TABLE I: Cross section for $\theta = 21°, 23°, 25°$ corresponding to $Q^2 \sim$ 1.3, 1.5 and 1.7 GeV$^2$ respectively. The cross section ($\frac{d\sigma}{dE'd\Omega}$) for each $x_B$ is in units of $\frac{nb}{sr\cdot MeV}$. Column 3, 4, 5 are statistical, systematic, and total uncertainties, respectively. The 2.7% (for $^{40}$Ca) and 3.0% (for $^{48}$Ca) normalization uncertainty are not included in the table.

| $x_B$ | theta [°] | $\sigma(^{40}$Ca) | Stat. uncert.[%] | Syst. uncert.[%] | Total uncert.[%] | $\sigma(^{48}$Ca) | Stat. uncert.[%] | Syst. uncert.[%] | Total uncert.[%] |
|---|---|---|---|---|---|---|---|---|---|
| 1.30 | 21 | 5.77E-01 | 0.6 | 1.9 | 2.0 | 6.30E-01 | 0.7 | 2.1 | 2.2 |
| 1.34 | 21 | 4.92E-01 | 0.6 | 1.9 | 2.0 | 5.43E-01 | 0.7 | 2.1 | 2.2 |
| 1.38 | 21 | 4.21E-01 | 0.6 | 1.9 | 2.0 | 4.69E-01 | 0.7 | 2.1 | 2.2 |
| 1.42 | 21 | 3.56E-01 | 0.6 | 1.9 | 2.0 | 3.98E-01 | 0.7 | 2.1 | 2.2 |
| 1.46 | 21 | 3.01E-01 | 0.7 | 1.9 | 2.0 | 3.43E-01 | 0.7 | 2.1 | 2.2 |
| 1.50 | 21 | 2.57E-01 | 0.7 | 1.9 | 2.0 | 2.92E-01 | 0.8 | 2.1 | 2.2 |
| 1.54 | 21 | 2.19E-01 | 0.7 | 1.9 | 2.0 | 2.54E-01 | 0.8 | 2.1 | 2.2 |
| 1.58 | 21 | 1.88E-01 | 0.8 | 1.9 | 2.1 | 2.17E-01 | 0.9 | 2.1 | 2.3 |
| 1.62 | 21 | 1.61E-01 | 0.9 | 1.9 | 2.1 | 1.88E-01 | 1.0 | 2.1 | 2.3 |
| 1.66 | 21 | 1.41E-01 | 1.0 | 1.9 | 2.2 | 1.66E-01 | 1.2 | 2.1 | 2.4 |
| 1.70 | 21 | 1.23E-01 | 1.1 | 1.9 | 2.2 | 1.41E-01 | 1.3 | 2.1 | 2.4 |
| 1.74 | 21 | 1.09E-01 | 1.4 | 1.9 | 2.4 | 1.26E-01 | 1.6 | 2.1 | 2.6 |
| 1.78 | 21 | 9.67E-02 | 1.6 | 1.9 | 2.5 | 1.12E-01 | 1.8 | 2.1 | 2.8 |
| 1.82 | 21 | 8.48E-02 | 1.8 | 1.9 | 2.6 | 1.01E-01 | 2.1 | 2.1 | 2.9 |
| 1.86 | 21 | 7.59E-02 | 2.5 | 1.9 | 3.1 | 8.86E-02 | 2.7 | 2.1 | 3.5 |
| 1.90 | 21 | 6.65E-02 | 2.7 | 1.9 | 3.3 | 7.81E-02 | 3.1 | 2.1 | 3.7 |
| 1.94 | 21 | 5.93E-02 | 3.0 | 1.9 | 3.6 | 6.93E-02 | 3.4 | 2.1 | 3.9 |
| 1.98 | 21 | 4.97E-02 | 2.9 | 1.9 | 3.5 | 5.95E-02 | 3.3 | 2.1 | 3.9 |
| 1.38 | 23 | 1.70E-01 | 0.7 | 1.9 | 2.0 | 1.90E-01 | 0.8 | 2.1 | 2.2 |
| 1.42 | 23 | 1.43E-01 | 0.8 | 1.9 | 2.0 | 1.60E-01 | 0.8 | 2.1 | 2.3 |
| 1.46 | 23 | 1.19E-01 | 0.8 | 1.9 | 2.0 | 1.34E-01 | 0.8 | 2.1 | 2.3 |
| 1.50 | 23 | 9.86E-02 | 0.8 | 1.9 | 2.1 | 1.16E-01 | 0.9 | 2.1 | 2.3 |
| 1.54 | 23 | 8.36E-02 | 0.8 | 1.9 | 2.1 | 9.69E-02 | 0.9 | 2.1 | 2.3 |
| 1.58 | 23 | 7.12E-02 | 0.9 | 1.9 | 2.1 | 8.20E-02 | 1.0 | 2.1 | 2.3 |
| 1.62 | 23 | 6.10E-02 | 1.0 | 1.9 | 2.2 | 7.14E-02 | 1.1 | 2.1 | 2.4 |
| 1.66 | 23 | 5.15E-02 | 1.1 | 1.9 | 2.2 | 6.06E-02 | 1.2 | 2.1 | 2.4 |

*Continued on next page*

TABLE I – *Continued from previous page*

| $x_B$ | theta [°] | $\sigma(^{40}Ca)$ | Stat. uncert.[%] | Syst. uncert.[%] | Total uncert.[%] | $\sigma(^{48}Ca)$ | Stat. uncert.[%] | Syst. uncert.[%] | Total uncert.[%] |
|---|---|---|---|---|---|---|---|---|---|
| 1.70 | 23 | 4.51E-02 | 1.1 | 1.9 | 2.2 | 5.20E-02 | 1.3 | 2.1 | 2.4 |
| 1.74 | 23 | 3.96E-02 | 1.4 | 1.9 | 2.3 | 4.54E-02 | 1.5 | 2.1 | 2.6 |
| 1.78 | 23 | 3.37E-02 | 1.5 | 1.9 | 2.4 | 4.03E-02 | 1.7 | 2.1 | 2.7 |
| 1.82 | 23 | 2.97E-02 | 1.6 | 1.9 | 2.5 | 3.48E-02 | 1.7 | 2.1 | 2.7 |
| 1.86 | 23 | 2.70E-02 | 2.2 | 1.9 | 2.9 | 3.17E-02 | 2.4 | 2.1 | 3.2 |
| 1.90 | 23 | 2.41E-02 | 2.7 | 1.9 | 3.3 | 2.81E-02 | 3.0 | 2.1 | 3.6 |
| 1.94 | 23 | 2.05E-02 | 2.9 | 1.9 | 3.5 | 2.42E-02 | 3.2 | 2.1 | 3.8 |
| 1.98 | 23 | 1.75E-02 | 3.0 | 1.9 | 3.6 | 2.03E-02 | 3.3 | 2.1 | 3.9 |
| 2.05 | 23 | 1.52E-02 | 1.3 | 1.9 | 2.3 | 1.79E-02 | 1.5 | 2.1 | 2.6 |
| 2.15 | 23 | 1.15E-02 | 1.4 | 1.9 | 2.4 | 1.34E-02 | 1.6 | 2.1 | 2.6 |
| 2.25 | 23 | 9.00E-03 | 1.6 | 1.9 | 2.5 | 1.07E-02 | 1.8 | 2.1 | 2.8 |
| 2.35 | 23 | 7.04E-03 | 1.9 | 1.9 | 2.7 | 8.04E-03 | 2.0 | 2.1 | 2.9 |
| 2.45 | 23 | 5.50E-03 | 2.1 | 1.9 | 2.9 | 6.34E-03 | 2.4 | 2.1 | 3.2 |
| 2.55 | 23 | 4.20E-03 | 2.4 | 1.9 | 3.0 | 4.93E-03 | 2.6 | 2.1 | 3.4 |
| 2.65 | 23 | 3.51E-03 | 2.8 | 1.9 | 3.4 | 4.17E-03 | 3.2 | 2.1 | 3.8 |
| 2.75 | 23 | 2.64E-03 | 3.1 | 1.9 | 3.6 | 3.32E-03 | 3.6 | 2.1 | 4.1 |
| 2.85 | 23 | 2.09E-03 | 3.5 | 1.9 | 4.0 | 2.66E-03 | 4.1 | 2.1 | 4.6 |
| 2.95 | 23 | 1.73E-03 | 4.0 | 1.9 | 4.4 | 2.18E-03 | 4.6 | 2.1 | 5.1 |
| 0.90 | 25 | 4.40E-01 | 0.4 | 1.9 | 1.9 | 4.86E-01 | 0.6 | 2.1 | 2.2 |
| 0.94 | 25 | 4.21E-01 | 0.4 | 1.9 | 1.9 | 4.53E-01 | 0.5 | 2.1 | 2.2 |
| 0.98 | 25 | 3.99E-01 | 0.4 | 1.9 | 1.9 | 4.19E-01 | 0.5 | 2.1 | 2.2 |
| 1.02 | 25 | 3.62E-01 | 0.4 | 1.9 | 1.9 | 3.80E-01 | 0.5 | 2.1 | 2.2 |
| 1.06 | 25 | 3.21E-01 | 0.5 | 1.9 | 2.0 | 3.38E-01 | 0.7 | 2.1 | 2.2 |
| 1.10 | 25 | 2.77E-01 | 0.6 | 1.9 | 2.0 | 2.92E-01 | 0.8 | 2.1 | 2.3 |
| 1.14 | 25 | 2.37E-01 | 0.8 | 1.9 | 2.0 | 2.53E-01 | 1.1 | 2.1 | 2.4 |
| 1.18 | 25 | 2.04E-01 | 0.5 | 1.9 | 2.0 | 2.21E-01 | 0.6 | 2.1 | 2.2 |
| 1.22 | 25 | 1.74E-01 | 0.6 | 1.9 | 2.0 | 1.89E-01 | 0.7 | 2.1 | 2.2 |
| 1.26 | 25 | 1.43E-01 | 0.6 | 1.9 | 2.0 | 1.57E-01 | 0.7 | 2.1 | 2.2 |
| 1.30 | 25 | 1.18E-01 | 0.7 | 1.9 | 2.0 | 1.32E-01 | 0.8 | 2.1 | 2.2 |
| 1.34 | 25 | 9.68E-02 | 0.8 | 1.9 | 2.1 | 1.08E-01 | 0.9 | 2.1 | 2.3 |
| 1.38 | 25 | 7.81E-02 | 1.0 | 1.9 | 2.1 | 8.93E-02 | 1.1 | 2.1 | 2.4 |
| 1.42 | 25 | 6.33E-02 | 1.4 | 1.9 | 2.4 | 7.22E-02 | 1.6 | 2.1 | 2.6 |
| 1.46 | 25 | 5.12E-02 | 0.7 | 1.9 | 2.0 | 5.86E-02 | 0.7 | 2.1 | 2.2 |
| 1.50 | 25 | 4.26E-02 | 0.8 | 1.9 | 2.0 | 4.77E-02 | 0.8 | 2.1 | 2.2 |
| 1.54 | 25 | 3.48E-02 | 0.8 | 1.9 | 2.1 | 4.05E-02 | 0.8 | 2.1 | 2.2 |
| 1.58 | 25 | 2.97E-02 | 0.9 | 1.9 | 2.1 | 3.35E-02 | 0.9 | 2.1 | 2.3 |
| 1.62 | 25 | 2.53E-02 | 1.0 | 1.9 | 2.1 | 2.84E-02 | 0.9 | 2.1 | 2.3 |
| 1.66 | 25 | 2.08E-02 | 1.0 | 1.9 | 2.2 | 2.42E-02 | 1.0 | 2.1 | 2.3 |
| 1.70 | 25 | 1.76E-02 | 1.1 | 1.9 | 2.2 | 2.11E-02 | 1.1 | 2.1 | 2.3 |
| 1.74 | 25 | 1.55E-02 | 1.2 | 1.9 | 2.3 | 1.78E-02 | 1.2 | 2.1 | 2.4 |
| 1.78 | 25 | 1.34E-02 | 1.4 | 1.9 | 2.3 | 1.54E-02 | 1.3 | 2.1 | 2.4 |
| 1.82 | 25 | 1.19E-02 | 1.5 | 1.9 | 2.4 | 1.36E-02 | 1.4 | 2.1 | 2.5 |
| 1.86 | 25 | 1.03E-02 | 1.6 | 1.9 | 2.5 | 1.20E-02 | 1.5 | 2.1 | 2.6 |
| 1.90 | 25 | 9.26E-03 | 2.0 | 1.9 | 2.7 | 1.06E-02 | 1.8 | 2.1 | 2.8 |
| 1.94 | 25 | 7.96E-03 | 2.3 | 1.9 | 3.0 | 8.89E-03 | 2.1 | 2.1 | 3.0 |
| 1.98 | 25 | 6.62E-03 | 2.6 | 1.9 | 3.2 | 7.80E-03 | 2.4 | 2.1 | 3.2 |

TABLE II: Per-nucleon cross section ratio, $\frac{\sigma(^{48}Ca)/48}{\sigma(^{40}Ca)/40}$, as function of $x_B$ for the combined data from all three scattering angles. Columns 3, 4, 5 are statistic, systematic, and total uncertainty, respectively. We only focus on the ratio up to $x_B = 2$ in this paper. The 1% normalization uncertainty is not included in this table.

| $x_B$ | $\frac{\sigma(^{48}Ca)/48}{\sigma(^{40}Ca)/40}$ | Statistical uncert.[%] | Systemmatic uncert.[%] | Total uncert.[%] |
|---|---|---|---|---|
| 0.90 | 0.921 | 0.003 | 0.008 | 0.009 |
| 0.94 | 0.897 | 0.003 | 0.008 | 0.009 |
| 0.98 | 0.875 | 0.003 | 0.008 | 0.008 |
| 1.02 | 0.873 | 0.003 | 0.008 | 0.008 |
| 1.06 | 0.878 | 0.004 | 0.008 | 0.009 |
| 1.10 | 0.878 | 0.005 | 0.008 | 0.010 |
| 1.14 | 0.888 | 0.007 | 0.008 | 0.011 |
| 1.18 | 0.903 | 0.004 | 0.008 | 0.009 |
| 1.22 | 0.907 | 0.004 | 0.008 | 0.009 |
| 1.26 | 0.914 | 0.005 | 0.008 | 0.010 |
| 1.30 | 0.913 | 0.002 | 0.008 | 0.008 |
| 1.34 | 0.920 | 0.002 | 0.008 | 0.009 |
| 1.38 | 0.930 | 0.002 | 0.008 | 0.009 |
| 1.42 | 0.933 | 0.003 | 0.008 | 0.009 |
| 1.46 | 0.948 | 0.003 | 0.009 | 0.009 |
| 1.50 | 0.951 | 0.003 | 0.009 | 0.009 |
| 1.54 | 0.965 | 0.003 | 0.009 | 0.009 |
| 1.58 | 0.961 | 0.003 | 0.009 | 0.009 |
| 1.62 | 0.973 | 0.004 | 0.009 | 0.010 |
| 1.66 | 0.980 | 0.004 | 0.009 | 0.010 |
| 1.70 | 0.965 | 0.004 | 0.009 | 0.010 |
| 1.74 | 0.965 | 0.005 | 0.009 | 0.010 |
| 1.78 | 0.973 | 0.005 | 0.009 | 0.010 |
| 1.82 | 0.986 | 0.006 | 0.009 | 0.011 |
| 1.86 | 0.980 | 0.007 | 0.009 | 0.011 |
| 1.90 | 0.978 | 0.008 | 0.009 | 0.012 |
| 1.94 | 0.976 | 0.009 | 0.009 | 0.013 |
| 1.98 | 0.987 | 0.010 | 0.009 | 0.013 |

TABLE III: The same as Table **??** for only angle $\theta = 21^\circ$.

| $x_B$ | $\frac{\sigma(^{48}Ca)/48}{\sigma(^{40}Ca)/40}$ | Statistical uncert.[%] | Systemmatic uncert.[%] | Total uncert.[%] |
|---|---|---|---|---|
| 1.30 | 0.910 | 0.002 | 0.008 | 0.008 |
| 1.34 | 0.919 | 0.002 | 0.008 | 0.009 |
| 1.38 | 0.927 | 0.003 | 0.008 | 0.009 |
| 1.42 | 0.933 | 0.003 | 0.008 | 0.009 |
| 1.46 | 0.948 | 0.003 | 0.009 | 0.009 |
| 1.50 | 0.950 | 0.003 | 0.009 | 0.009 |
| 1.54 | 0.964 | 0.004 | 0.009 | 0.009 |
| 1.58 | 0.966 | 0.004 | 0.009 | 0.010 |
| 1.62 | 0.979 | 0.004 | 0.009 | 0.010 |
| 1.66 | 0.982 | 0.005 | 0.009 | 0.010 |
| 1.70 | 0.961 | 0.005 | 0.009 | 0.010 |
| 1.74 | 0.968 | 0.006 | 0.009 | 0.010 |
| 1.78 | 0.970 | 0.006 | 0.009 | 0.011 |
| 1.82 | 0.993 | 0.007 | 0.009 | 0.012 |
| 1.86 | 0.981 | 0.008 | 0.009 | 0.012 |
| 1.90 | 0.984 | 0.009 | 0.009 | 0.013 |
| 1.94 | 0.982 | 0.011 | 0.009 | 0.014 |
| 1.98 | 0.998 | 0.013 | 0.009 | 0.016 |

TABLE IV: The same as Table **??** for only angle $\theta = 23°$.

| $x_B$ | $\frac{\sigma(^{48}Ca)/48}{\sigma(^{40}Ca)/40}$ | Statistical uncert.[%] | Systemmatic uncert.[%] | Total uncert.[%] |
|---|---|---|---|---|
| 1.38 | 0.933 | 0.005 | 0.008 | 0.010 |
| 1.42 | 0.929 | 0.006 | 0.008 | 0.010 |
| 1.46 | 0.941 | 0.006 | 0.008 | 0.011 |
| 1.50 | 0.978 | 0.007 | 0.009 | 0.011 |
| 1.54 | 0.967 | 0.008 | 0.009 | 0.012 |
| 1.58 | 0.960 | 0.009 | 0.009 | 0.012 |
| 1.62 | 0.976 | 0.010 | 0.009 | 0.013 |
| 1.66 | 0.982 | 0.011 | 0.009 | 0.014 |
| 1.70 | 0.959 | 0.011 | 0.009 | 0.014 |
| 1.74 | 0.956 | 0.013 | 0.009 | 0.015 |
| 1.78 | 0.997 | 0.014 | 0.009 | 0.017 |
| 1.82 | 0.977 | 0.015 | 0.009 | 0.018 |
| 1.86 | 0.980 | 0.017 | 0.009 | 0.020 |
| 1.90 | 0.969 | 0.020 | 0.009 | 0.022 |
| 1.94 | 0.984 | 0.024 | 0.009 | 0.026 |
| 1.98 | 0.965 | 0.018 | 0.009 | 0.020 |

TABLE V: The same as Table **??** for only angle $\theta = 25°$.

| $x_B$ | $\frac{\sigma(^{48}Ca)/48}{\sigma(^{40}Ca)/40}$ | Statistical uncert.[%] | Systemmatic uncert.[%] | Total uncert.[%] |
|---|---|---|---|---|
| 0.90 | 0.921 | 0.003 | 0.008 | 0.009 |
| 0.94 | 0.897 | 0.003 | 0.008 | 0.009 |
| 0.98 | 0.875 | 0.003 | 0.008 | 0.008 |
| 1.02 | 0.873 | 0.003 | 0.008 | 0.008 |
| 1.06 | 0.878 | 0.004 | 0.008 | 0.009 |
| 1.10 | 0.878 | 0.005 | 0.008 | 0.010 |
| 1.14 | 0.888 | 0.007 | 0.008 | 0.011 |
| 1.18 | 0.903 | 0.004 | 0.008 | 0.009 |
| 1.22 | 0.907 | 0.004 | 0.008 | 0.009 |
| 1.26 | 0.914 | 0.005 | 0.008 | 0.010 |
| 1.30 | 0.935 | 0.006 | 0.008 | 0.010 |
| 1.34 | 0.926 | 0.007 | 0.008 | 0.011 |
| 1.38 | 0.953 | 0.009 | 0.009 | 0.012 |
| 1.42 | 0.949 | 0.011 | 0.009 | 0.014 |
| 1.46 | 0.955 | 0.007 | 0.009 | 0.011 |
| 1.50 | 0.932 | 0.007 | 0.008 | 0.011 |
| 1.54 | 0.969 | 0.009 | 0.009 | 0.012 |
| 1.58 | 0.938 | 0.009 | 0.008 | 0.013 |
| 1.62 | 0.934 | 0.010 | 0.008 | 0.013 |
| 1.66 | 0.973 | 0.012 | 0.009 | 0.015 |
| 1.70 | 0.999 | 0.013 | 0.009 | 0.016 |
| 1.74 | 0.960 | 0.014 | 0.009 | 0.017 |
| 1.78 | 0.962 | 0.016 | 0.009 | 0.018 |
| 1.82 | 0.957 | 0.017 | 0.009 | 0.019 |
| 1.86 | 0.972 | 0.019 | 0.009 | 0.021 |
| 1.90 | 0.957 | 0.022 | 0.009 | 0.023 |
| 1.94 | 0.930 | 0.026 | 0.008 | 0.027 |
| 1.98 | 0.982 | 0.033 | 0.009 | 0.034 |
